# Supplementary material for: Control-R: Towards controllable test-time scaling
Source: arXiv:2506.00189 source file (2025-05-30)
Supplement: Supplementary file 1 [file Details_of_R1-distillation-kit.tex]

\section{Details of R1-distillation-kit}
